# Supplementary material for: Causality on Cross-Sectional Data: Stable Specification Search in Constrained Structural Equation Modeling
Source: arXiv:1506.05600 source file (2016-07-14)

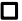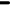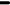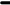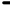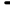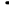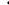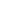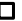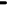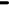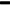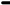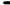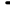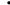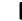

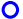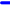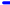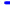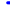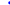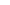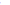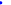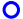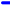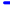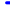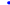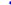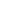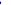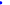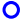

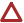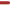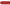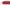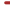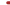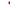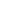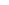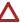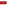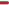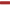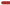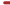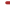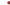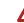

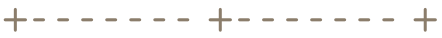

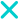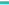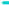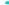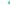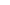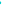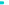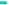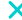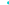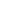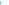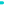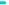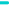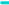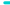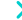

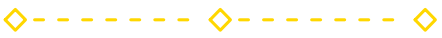

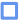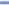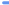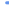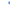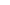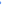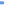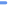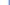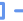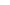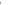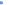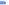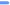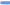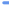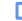

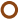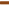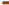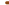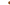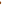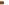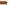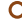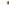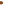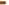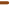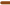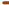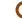



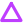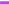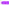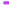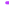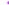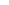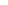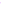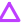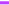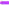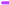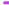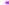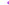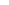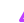

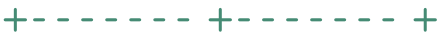

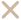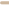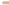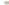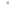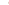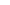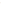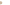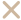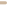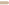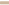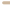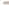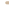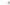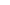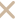

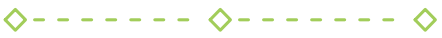

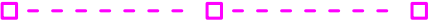

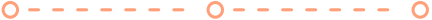

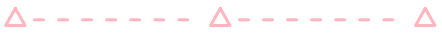

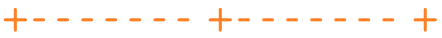



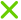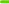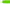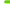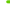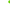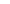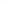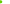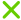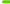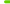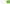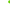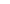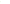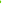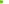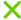

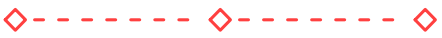

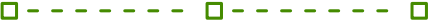

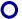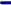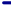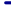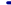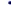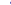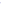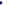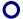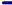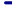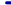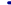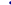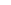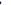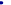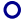

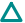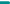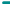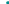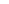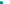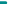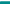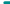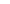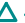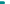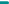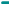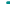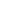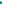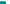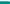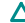

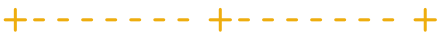

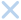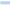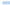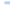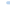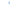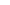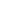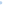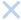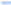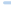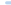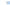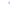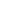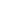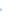

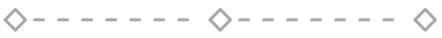



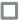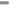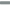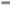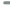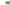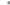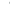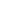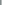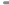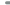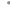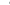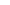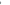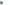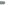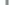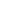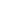

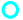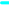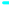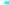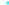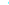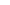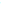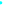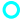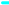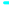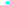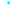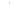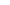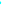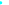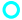

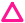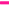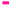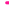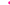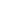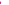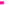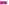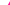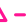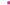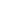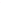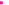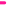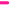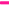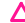

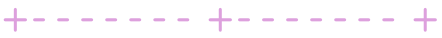

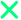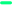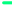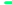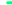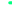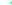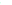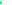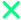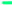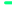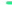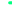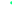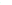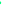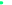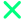

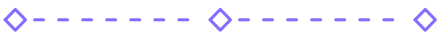

Supplement: Supplementary file 3 [file appendixCFSCausals.pdf]
