# Supplementary material for: Causality on Cross-Sectional Data: Stable Specification Search in Constrained Structural Equation Modeling
Source: arXiv:1506.05600 source file (2016-07-14)

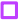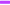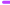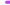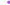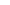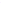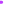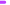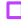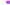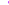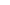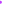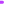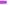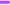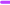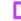

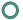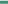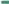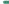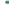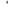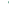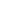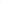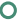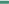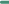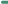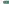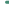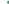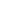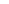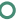

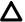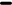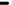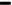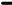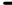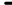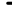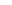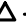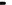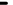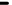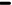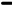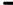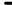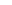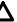

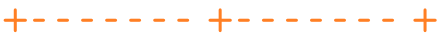

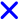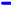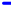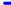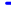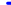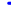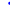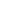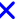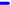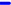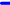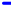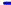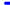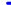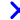

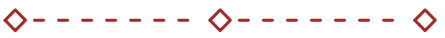

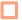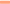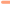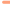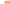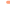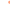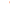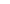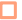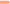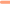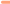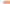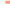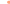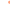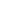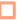

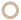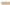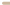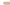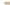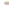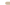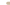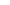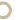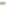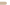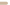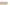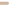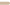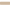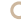



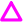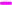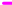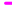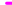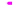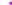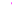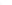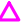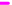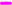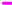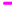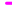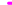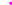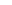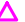

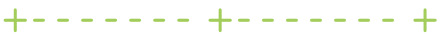

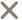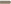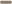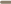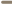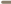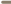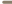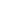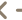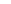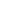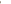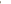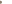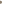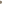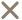

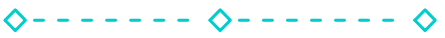

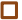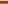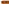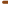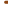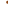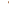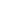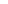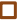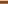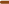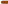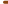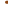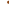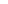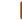

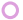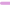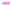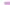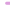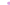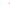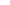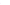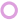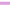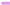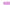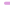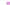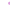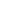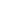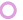

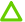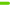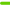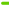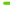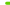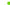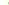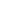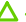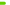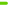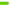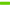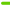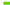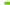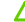

Supplement: Supplementary file 4 [file appendixCFSEdges.pdf]
